# Supplementary material for: Relativistic coupled cluster with completely renormalized and perturbative triples corrections
Source: arXiv:2404.13231 ancillary file (2024-06-19)
Supplement: Supplementary file 1 [file x2c_crcc_SI.pdf]

# Supporting Information for: Relativistic coupled cluster with completely renormalized and perturbative triples corrections

Stephen H. Yuwono,[†] Run R. Li,[†] Tianyuan Zhang,[‡] Kshitijkumar Surjuse,[¶] Edward F. Valeev,[¶] Xiaosong Li,[*,‡] and A. Eugene DePrince III[*,†]

† *Department of Chemistry and Biochemistry, Florida State University, Tallahassee, FL 32306-4390, USA*

‡*Department of Chemistry, University of Washington, Seattle, WA 98195, USA*

¶*Department of Chemistry, Virginia Tech, Blacksburg, VA 24061, USA*

E-mail: xsli@uw.edu; adeprince@fsu.edu

# S1 Total Electronic Energies Data

This Supporting Information is accompanied by a collection of CSV files that can be used to reproduce our data:

- `[name]_[relativistic-type]_[basis]_[kramers-type].csv`: twenty CSV files containing the total electronic energies used to construct the PECs shown in Figs. 1–4 of the main text.

- `basis_set_analysis.csv`: one CSV file that contains the necessary information to replicate the basis set analysis performed in Table 7 of the main text.

# S2 Fit Information And Additional Spectroscopic Parameters

The spectroscopic parameters ($D_\mathrm{e}$, $R_\mathrm{e}$, and $\omega_\mathrm{e}$) reported in the main text is obtained by fitting a total of 5 points around the minimum energy point (*i.e.*, including the energies at two shorter and two longer grid points) of each of the PECs to a 4th-order polynomial

$$E(R) = aR^4 + bR^3 + cR^2 + dR + e, \tag{1}$$

where $E(R)$ is the energy in hartree and $R$ is the interatomic distance in Å. The $R_\mathrm{e}$ value and its corresponding energy (used for $D_\mathrm{e}$ computation) were subsequently determined using the fit at grid points that are $10^{-3}$ Å apart. The values of $\omega_\mathrm{e}$ and $\omega_\mathrm{e}\chi_\mathrm{e}$ (both in cm$^{-1}$) were computed as

$$\omega_\mathrm{e} = 5.3088375 \times 10^{-11} \sqrt{\frac{k_2}{\mu}} \tag{2}$$

and

$$\omega_\mathrm{e}\chi_\mathrm{e} = 1.2415491 \times 10^{-6} \left(\frac{\omega_\mathrm{e}}{k_2}\right)^2 \left(\frac{5.0k_3^2}{3.0k_2} - k_4\right), \tag{3}$$

respectively, where $k_n$ is the $n$-th derivative of $E(R)$ in attojoule/Å$^n$ and $\mu$ is the reduced mass of the dimer in kg. The units and constant that we used follow the convention in Psi4's `anharmonicity` function (see `https://github.com/psi4/psi4/blob/master/psi4/driver/diatomic.py` – last accessed June 12, 2024), for reproducibility purposes. In addition to the spectroscopic data reported in the main text, we report here the anharmonicity constant ($\omega_e\chi_e$) and bond dissociation energy ($D_0$) of each PEC, along with the fit parameters.

**Table S1: Anharmonicity constant ($\omega_e\chi_e$) and bond dissociation energy ($D_0$) for $Cu_2$ using the ANO-RCC-VDZP basis set. All values are reported as deviations from experimentally-obtained values.**

| Method | $\omega_e\chi_e$ (cm$^{-1}$) | | | $D_0$ (eV)[1] | | |
|---|---|---|---|---|---|---|
| | GHF | SF-1eX2C | 1eX2C | GHF | SF-1eX2C | 1eX2C |
| CCSD | −0.079 | −0.043 | −0.044 | −0.24 (0.24) | −0.14 (0.37) | −0.13 (0.38) |
| CCSD(T) | 0.137 | 0.149 | 0.149 | −0.12 (−0.36) | −0.01 (−0.27) | 0.00 (−0.26) |
| CR-CC(2,3)$_A$ | 0.096 | 0.140 | 0.139 | −0.11 (0.04) | 0.01 (0.17) | 0.02 (0.18) |
| CR-CC(2,3)$_B$ | 0.091 | 0.122 | 0.121 | −0.13 (0.06) | 0.00 (0.20) | 0.00 (0.20) |
| CR-CC(2,3)$_C$ | 0.078 | −0.098 | 1.093 | −0.13 (0.03) | −0.02 (0.16) | 0.00 (0.17) |
| CR-CC(2,3)$_D$ | 0.077 | −0.120 | 1.109 | −0.13 (0.04) | −0.01 (0.18) | 0.00 (0.19) |
| Experiment[2] | | 1.04215 | | | 2.00 | |

[1]The numbers outside and inside parentheses refer to Kramers-unrestricted and restricted dissociation energies, respectively.
[2]Ref. 124.

**Table S2: Anharmonicity constant ($\omega_e\chi_e$) and bond dissociation energy ($D_0$) for $Ag_2$ using the ANO-RCC-VDZP basis set. All values are reported as deviations from experimentally-obtained values.**

| Method | $\omega_e\chi_e$ (cm$^{-1}$) | | | $D_0$ (eV)[1] | | |
|---|---|---|---|---|---|---|
| | GHF | SF-1eX2C | 1eX2C | GHF | SF-1eX2C | 1eX2C |
| CCSD | 0.268 | −0.099 | −0.078 | 0.70 (1.21) | −0.12 (0.61) | −0.04 (0.69) |
| CCSD(T) | 0.320 | −0.002 | 0.016 | 0.82 (0.61) | 0.01 (−0.28) | 0.08 (−0.21) |
| CR-CC(2,3)$_A$ | 0.309 | −0.019 | 0.000 | 0.80 (0.92) | −0.01 (0.18) | 0.07 (0.26) |
| CR-CC(2,3)$_B$ | 0.306 | −0.022 | −0.003 | 0.80 (0.95) | −0.02 (0.24) | 0.06 (0.32) |
| CR-CC(2,3)$_C$ | 0.351 | 0.156 | 0.057 | 0.80 (0.88) | −0.01 (0.14) | 0.07 (0.22) |
| CR-CC(2,3)$_D$ | 0.352 | 0.155 | 0.058 | 0.80 (0.89) | −0.01 (0.15) | 0.07 (0.23) |
| Experiment[2] | | 0.60 | | | 1.65 | |

[1]The numbers outside and inside parentheses refer to Kramers-unrestricted and restricted dissociation energies, respectively.
[2]Ref. 114.

**Table S3: Anharmonicity constant ($\omega_e\chi_e$) and bond dissociation energy ($D_0$) for $Au_2$ using the ANO-RCC-VDZP basis set. All values are reported as deviations from experimentally-obtained values.**

| Method | $\omega_e\chi_e$ (cm$^{-1}$) | | | $D_0$ (eV)[1] | | |
|---|---|---|---|---|---|---|
| | GHF | SF-1eX2C | 1eX2C | GHF | SF-1eX2C | 1eX2C |
| CCSD | 0.776 | 0.059 | 0.045 | 30.94 (32.21) | 0.00 (1.09) | 0.81 (1.88) |
| CCSD(T) | 0.975 | 0.087 | −0.072 | 31.30 (32.03) | 0.17 (−0.16) | 0.97 (0.64) |
| CR-CC(2,3)$_A$ | —[2] | 0.079 | −0.076 | —[2] | 0.16 (0.45) | 0.96 (1.25) |
| CR-CC(2,3)$_B$ | —[2] | 0.077 | −0.078 | —[2] | 0.15 (0.55) | 0.95 (1.35) |
| CR-CC(2,3)$_C$ | —[2] | 0.036 | 0.045 | —[2] | 0.15 (0.40) | 0.96 (1.19) |
| CR-CC(2,3)$_D$ | —[2] | 0.035 | 0.047 | —[2] | 0.15 (0.43) | 0.96 (1.22) |
| Experiment[3] | | 0.42 | | | 2.29 | |

[1]The numbers outside and inside parentheses refer to Kramers-unrestricted and restricted dissociation energies, respectively.
[2]Calculations not performed because the reference curve has a significantly wrong shape compared to the expected result.
[3]Refs. 114, 134, 135, 141.

**Table S4: Comparison between the anharmonicity constant ($\omega_e\chi_e$) and bond dissociation energy ($D_0$) of $Au_2$ obtained using the ANO-RCC-VDZP (ANO) and x2c-SVPall-2c (SVP) basis sets. All values are reported as deviations from experimentally-obtained values.**

| Method | $\omega_e\chi_e$ (cm$^{-1}$) | | $D_0$ (eV)[1] | |
|---|---|---|---|---|
| | ANO[2] | SVP | ANO[2] | SVP |
| SF-1eX2C-CCSD | 0.059 | −0.122 | 0.00 | −0.14 |
| SF-1eX2C-CCSD(T) | 0.087 | −0.103 | 0.17 | 0.00 |
| 1eX2C-CCSD | 0.045 | −0.153 | 0.81 | −0.02 |
| 1eX2C-CCSD(T) | −0.072 | −0.135 | 0.97 | 0.13 |
| Experiment[3] | 0.42 | | 2.29 | |

[1]Kramers-unrestricted dissociation energies.
[2]Taken from Table S3.
[3]Refs. 114, 134, 135, 141.

**Table S5: Fit parameters for $Cu_2$ using the ANO-RCC-VDZP basis set.**

| Method | *a* | *b* | *c* | *d* | *e* |
|---|---|---|---|---|---|
| | | | GHF | | |
| CCSD | 1.88886418E-01 | -1.90455534E+00 | 7.25937964E+00 | -1.23549375E+01 | -3.25580024E+03 |
| CCSD(T) | 1.79629583E-01 | -1.82178571E+00 | 6.97829382E+00 | -1.19211993E+01 | -3.25608186E+03 |
| CR-CC(2,3)$_A$ | 1.83762834E-01 | -1.85947905E+00 | 7.10816051E+00 | -1.21211107E+01 | -3.25596801E+03 |
| CR-CC(2,3)$_B$ | 1.82589875E-01 | -1.84877338E+00 | 7.07179304E+00 | -1.20670771E+01 | -3.25599598E+03 |
| CR-CC(2,3)$_C$ | 2.14599874E-01 | -2.14475837E+00 | 8.09712234E+00 | -1.36429879E+01 | -3.25509388E+03 |
| CR-CC(2,3)$_D$ | 2.14847792E-01 | -2.14705810E+00 | 8.10514395E+00 | -1.36554634E+01 | -3.25508656E+03 |
| | | | SF-1eX2C | | |
| CCSD | 2.61862001E-01 | -2.56220304E+00 | 9.47253061E+00 | -1.56389070E+01 | -3.29779183E+03 |
| CCSD(T) | 2.65322040E-01 | -2.59382219E+00 | 9.57638849E+00 | -1.57794370E+01 | -3.29775356E+03 |
| CR-CC(2,3)$_A$ | 2.63698000E-01 | -2.57980900E+00 | 9.53244910E+00 | -1.57198283E+01 | -3.29778545E+03 |
| CR-CC(2,3)$_B$ | 2.63406500E-01 | -2.57702847E+00 | 9.52283148E+00 | -1.57060460E+01 | -3.29779051E+03 |
| CR-CC(2,3)$_C$ | 2.94782208E-01 | -2.84929374E+00 | 1.04068687E+01 | -1.69775898E+01 | -3.29711205E+03 |
| CR-CC(2,3)$_D$ | 2.98413625E-01 | -2.88113720E+00 | 1.05114235E+01 | -1.71299438E+01 | -3.29702889E+03 |
| | | | 1eX2C | | |
| CCSD | 2.61742250E-01 | 2.56108068E+00 | 9.46859345E+00 | -1.56326586E+01 | -3.29775948E+03 |
| CCSD(T) | 2.65207499E-01 | 2.59275288E+00 | 9.57264688E+00 | -1.57734979E+01 | -3.29772103E+03 |
| CR-CC(2,3)$_A$ | 2.63577333E-01 | 2.57867982E+00 | 9.52849669E+00 | -1.57135760E+01 | -3.29775308E+03 |
| CR-CC(2,3)$_B$ | 2.63326333E-01 | 2.57626055E+00 | 9.52008521E+00 | -1.57015794E+01 | -3.29775715E+03 |
| CR-CC(2,3)$_C$ | 1.15816582E-01 | 1.29180626E+00 | 5.33353321E+00 | -9.64643082E+00 | -3.30104136E+03 |
| CR-CC(2,3)$_D$ | 1.12971250E-01 | 1.26698549E+00 | 5.25250302E+00 | -9.52910711E+00 | -3.30110490E+03 |

**Table S6: Fit parameters for $Ag_2$ using the ANO-RCC-VDZP basis set.**

| Method | *a* | *b* | *c* | *d* | *e* |
|---|---|---|---|---|---|
| | | | GHF | | |
| CCSD | 2.38159170E-01 | -2.58544170E+00 | 1.05777388E+01 | -1.92895665E+01 | -1.01449082E+04 |
| CCSD(T) | 2.38991377E-01 | -2.59455585E+00 | 1.06129034E+01 | -1.93436113E+01 | -1.01448999E+04 |
| CR-CC(2,3)$_A$ | 2.38620791E-01 | -2.59071914E+00 | 1.05985320E+01 | -1.93210385E+01 | -1.01449113E+04 |
| CR-CC(2,3)$_B$ | 2.38574628E-01 | -2.59020354E+00 | 1.05964687E+01 | -1.93176412E+01 | -1.01449126E+04 |
| CR-CC(2,3)$_C$ | 2.15003627E-01 | -2.35670391E+00 | 9.72983606E+00 | -1.78886494E+01 | -1.01457988E+04 |
| CR-CC(2,3)$_D$ | 2.14827423E-01 | -2.35498799E+00 | 9.72359031E+00 | -1.78785834E+01 | -1.01458049E+04 |
| | | | SF-1eX2C | | |
| CCSD | 2.52124920E-01 | -2.76906850E+00 | 1.14744362E+01 | -2.12232967E+01 | -1.06114064E+04 |
| CCSD(T) | 2.52883960E-01 | -2.77750282E+00 | 1.15059958E+01 | -2.12681387E+01 | -1.06114078E+04 |
| CR-CC(2,3)$_A$ | 2.52533917E-01 | -2.77379643E+00 | 1.14920134E+01 | -2.12459423E+01 | -1.06114193E+04 |
| CR-CC(2,3)$_B$ | 2.52501918E-01 | -2.77340988E+00 | 1.14904597E+01 | -2.12435654E+01 | -1.06114196E+04 |
| CR-CC(2,3)$_C$ | 2.14174750E-01 | -2.38753730E+00 | 1.00343605E+01 | -1.88022188E+01 | -1.06129573E+04 |
| CR-CC(2,3)$_D$ | 2.14097794E-01 | -2.38670523E+00 | 1.00310153E+01 | -1.87962851E+01 | -1.06129612E+04 |
| | | | 1eX2C | | |
| CCSD | 2.51083459E-01 | -2.75759447E+00 | 1.14269647E+01 | -2.11345973E+01 | -1.06105736E+04 |
| CCSD(T) | 2.51841166E-01 | -2.76601696E+00 | 1.14584911E+01 | -2.11794240E+01 | -1.06105750E+04 |
| CR-CC(2,3)$_A$ | 2.51492667E-01 | -2.76232662E+00 | 1.14445711E+01 | -2.11573340E+01 | -1.06105863E+04 |
| CR-CC(2,3)$_B$ | 2.51411210E-01 | -2.76144530E+00 | 1.14411633E+01 | -2.11518718E+01 | -1.06105886E+04 |
| CR-CC(2,3)$_C$ | 2.43171789E-01 | -2.67957062E+00 | 1.11360556E+01 | -2.06459485E+01 | -1.06109068E+04 |
| CR-CC(2,3)$_D$ | 2.42952918E-01 | -2.67736315E+00 | 1.11277275E+01 | -2.06320176E+01 | -1.06109155E+04 |

**Table S7: Fit parameters for $Au_2$ using the ANO-RCC-VDZP (ANO) and x2c-SVPall-2c (SVP) basis sets.**

| Method | *a* | *b* | *c* | *d* | *e* |
|---|---|---|---|---|---|
| | | | GHF/ANO | | |
| CCSD | 1.40137914E+01 | -1.20261854E+02 | 3.87490887E+02 | -5.54313287E+02 | -3.03902775E+04 |
| CCSD(T) | 1.27823799E+01 | -1.11348918E+02 | 3.63266643E+02 | -5.25032477E+02 | -3.04035731E+04 |
| | | | SF-1eX2C/ANO | | |
| CCSD | 3.86708698E-01 | -4.25676838E+00 | 1.76557849E+01 | -3.26235861E+01 | -3.79945420E+04 |
| CCSD(T) | 3.86502247E-01 | -4.25606766E+00 | 1.76537333E+01 | -3.26115239E+01 | -3.79945892E+04 |
| CR-CC(2,3)$_A$ | 3.85330198E-01 | -4.24298245E+00 | 1.76001196E+01 | -3.25150535E+01 | -3.79946537E+04 |
| CR-CC(2,3)$_B$ | 3.85479131E-01 | -4.24443053E+00 | 1.76056681E+01 | -3.25251246E+01 | -3.79946451E+04 |
| CR-CC(2,3)$_C$ | 4.62289584E-01 | -5.00718572E+00 | 2.04415858E+01 | -3.72033903E+01 | -3.79917604E+04 |
| CR-CC(2,3)$_D$ | 4.63505344E-01 | -5.01928506E+00 | 2.04867044E+01 | -3.72781012E+01 | -3.79917141E+04 |
| | | | 1eX2C/ANO | | |
| CCSD | 3.82587947E-01 | -4.20497363E+00 | 1.74151118E+01 | -3.21190238E+01 | -3.79721901E+04 |
| CCSD(T) | 5.68609504E-01 | -6.02934288E+00 | 2.41157300E+01 | -4.30400421E+01 | -3.79655536E+04 |
| CR-CC(2,3)$_A$ | 5.67046469E-01 | -6.01249672E+00 | 2.40486423E+01 | -4.29223204E+01 | -3.79656305E+04 |
| CR-CC(2,3)$_B$ | 5.67352325E-01 | -6.01545850E+00 | 2.40596408E+01 | -4.29410435E+01 | -3.79656170E+04 |
| CR-CC(2,3)$_C$ | 4.65878170E-01 | -5.03499995E+00 | 2.05108169E+01 | -3.72375562E+01 | -3.79690555E+04 |
| CR-CC(2,3)$_D$ | 4.64477368E-01 | -5.02146252E+00 | 2.04618332E+01 | -3.71589033E+01 | -3.79691027E+04 |
| | | | SF-1eX2C/SVP | | |
| CCSD | 3.57728633E-01 | -3.94420500E+00 | 1.64070610E+01 | -3.04595154E+01 | -3.79963155E+04 |
| CCSD(T) | 3.57841830E-01 | -3.94467400E+00 | 1.64031639E+01 | -3.04372837E+01 | -3.79963662E+04 |
| | | | 1eX2C/SVP | | |
| CCSD | 3.66434298E-01 | -4.01968792E+00 | 1.66387300E+01 | -3.07438221E+01 | -3.80302530E+04 |
| CCSD(T) | 3.66542138E-01 | -4.02009779E+00 | 1.66346361E+01 | -3.07213905E+01 | -3.80303038E+04 |
